# Supplementary material for: Efficient Methods for Non-stationary Online Learning
Source: arXiv:2309.08911 source file (2025-09-09)
Supplement: Supplementary file 1 [file appendix_proof_ppd_adaptive.tex]

%!TEX root = ../jmlr23_projection.tex
\section{Omitted Details for Partially Small-loss Adaptive Regret}
\label{sec:appendix-ppd-adaptive}
To illustrate the design of efficient adaptive algorithm more clearly, we here present a partially problem-dependent adaptive regret for convex and smooth functions, in which the base-algorithm and meta-algorithm are basically the same as specified in the main text while the geometric covering is much simpler.
We present this part to highlight the necessity of using Adapt-MLProd algorithm~\citep{COLT'14:second-order-Hedge} (a PEA algorithm with a \emph{second-order} regret guarantee) as the meta-algorithm to reduce the projection complexity for our proposal. 

\subsection{Algorithm and Theorem}

\begin{algorithm}[!t]
    \caption{Efficient Algorithm for Partially Problem-dependent Adaptive Regret}
    \label{alg:appendix-ppd-adaptive}
    \begin{algorithmic}[1]
        \REQUIRE base-algorithm (SOGD)
        \STATE{Let $\x_1$ be any point in $\X$.}
        \FOR{$t=1$ {\bfseries to} $T$}
            \STATE Receive the gradient information $\nabla f_t(\x_t)$.
            \STATE Construct the surrogate loss $g_t: \Y \mapsto \R$ according to~\pref{eq:surrogate-loss}. \label{line:alg-appendix-ppd surrogate loss}
            \STATE Compute the (sub-)gradient $\gradg_t(\y_t)$ according to Lemma~\ref{lemma:gradient-compute}.
            \STATE Remove base-learners whose ending time are $t+1$.
            \STATE Initialize a new base-learner with ending time $e_t = j$ satisfying $[t, j-1] \in \mathcal{C}$.
            \STATE Set $\gamma_t = \ln(j)$, $w_{t, t} = 1$, $\eta_{t, t} = \min\{1/2, \sqrt{\gamma_t} \}$
            \STATE Send $\gradg_t(\y_t)$ to all base-learners and obtain local predictions $\y_{t+1,i}$ for $i \in A_t$.
            \STATE Define $\hat{\ell}_t = \inner{\nabla g_t(\y_t)}{\y_t} / (2GD)$, $\ell_{t,i} = \inner{\nabla g_t(\y_t)}{\y_{t,i}}/(2GD), \forall i \in A_t.$
            \STATE Meta-algorithm updates the intermediate variables: for $i\in A_{t+1}$,
            \begin{equation}
                \label{eq:ppd-meta-adamlprod-inner}
                \eta_{t+1, i} = \min \Bigg\{\frac{1}{2}, \sqrt{\frac{\gamma_i}{1 + \sum_{k=s_i}^{t} (\hat{\ell}_k - \ell_{k, i})^2}} \Bigg\}, w_{t+1, i} = \Big(w_{t,i} \big(1 + \eta_{t,i} (\hat{\ell}_{t} - \ell_{t, i})\big) \Big)^{\frac{\eta_{t+1, i}}{\eta_{t, i}}}.
            \end{equation}
            \STATE Meta-algorithm updates weight $\p_{t+1} \in \Delta_{\abs{A_{t+1}}}$ by: $p_{t+1, i} = \frac{w_{t+1, i} \cdot \eta_{t+1, i}}{ \sum_{j \in A_{t+1}} w_{t+1, j} \cdot \eta_{t+1, j}} $, $i \in A_{t+1}$.
        
        \STATE Compute $\y_{t+1} = \sum_{i \in A_{t+1}} p_{t+1,i} \y_{t+1,i}$. \label{line:alg-appendix-ppd combine-y-adaptive}
            \STATE Submit $\x_{t+1} = \Pi_{\X}[\y_{t+1}]$. \LineComment{The only projection onto feasible domain $\X$ per round.}
        \ENDFOR
    \end{algorithmic}
\end{algorithm}

\pnote{describe the algorithm}

Substituting the PDCGC with the vanilla CGC will give the partially problem-dependent adaptive algorithm, which has the following guarantee,
\begin{myThm}
    \label{thm:adaptive-any-interval}
    Under Assumptions~\ref{assumption:bounded-gradient},~\ref{assumption:bounded-domain}, and~\ref{assumption:smoothness}, for any interval $I = [r, s] \subseteq [T]$, our proposed algorithm for partially problem-dependent adaptive regret (see Algorithm~\ref{algo:partial-pb-adaptive}) satisfies
    \begin{equation*}
        \sum_{\tau=r}^s f_\tau(\x_\tau) - \sum_{\tau = r}^s f_\tau(\u) \leq \O\left(\sqrt{F_I \log s \log (s-r)} \right),
    \end{equation*}
    for any comparator $\u \in \X$, where $F_I = \sum_{\tau = r}^s f_\tau(\u)$.

    If we further restrict the considered interval with length $|I| = \Omega(\log T)$, then our algorithm can achieve, 
    \begin{equation*}
        \sum_{\tau=r}^s f_\tau(\x_\tau) - \sum_{\tau = r}^s f_\tau(\u) \leq \O\left(\sqrt{F_I \log s \log (s-r)} \wedge \sqrt{|I| \log s} \right).
    \end{equation*}
\end{myThm}

\subsection{Key Lemmas}

To prove the preceding Theorem, several key lemmas are required. The next Lemma analyzes the base-regret in terms of the surrogate loss,
\begin{myLemma}
    \label{lemma:adaptive-surrogate-base-regret}
    Under Assumptions~\ref{assumption:bounded-domain}, and~\ref{assumption:smoothness}, for an interval in CGC $I = [i,j] \in \mathcal{C}$ and any $t \in [i,j]$, there exists an expert-algorithm $\Ecal_i$ satisfies
    \begin{equation*}
        \sum_{\tau=i}^t \inner{\gradg_t(\y_t)}{\y_{\tau, I} - \u} \leq 2D\sqrt{\delta} + 4D\sqrt{L\sum_{\tau=i}^t f_\tau(\x_\tau)},
    \end{equation*}
    for any comparator $\u \in \X$.
\end{myLemma}

The next Lemma gives the analysis for Adapt-ML-Prod\citep{COLT'14:second-order-Hedge} cooperated with CGC, which is guaranteed with second-order excess loss bound in adaptive setting.
\begin{myLemma}
    \label{lemma:adaptive-surrogate-meta-regret}
    Under Assumptions~\ref{assumption:bounded-domain}, and~\ref{assumption:smoothness}, for any interval in CGC $I=[i, j] \in \mathcal{C}$ and any $t \in [i, j]$, the surrogate meta-regret can be bounded as
    \begin{equation*}
        \sum_{\tau = i}^t \inner{\gradg_t(\y_t)}{\y_t - \y_{t, i}} \leq 8D\sqrt{L\ln(1+j) \sum_{\tau=i}^t f_t(\x_t)} + 16GD\ln(1+t) + 8GD\sqrt{\ln(1+t)}.
    \end{equation*}
\end{myLemma}

The last Lemma in this secion provides the regret upper bound for intervals lying in CGC, which can be seen as the mid-step to achieve adaptive regret regarding any interval.
\begin{myLemma}
    \label{lemma:adaptive-covering-regret}
    Under Assumptions~\ref{assumption:bounded-gradient},~\ref{assumption:bounded-domain}, and~\ref{assumption:smoothness}, for any interval in CGC $[i, j] \in \mathcal{C}$ and any $t \in [i, j]$, adaptive algorithm satisfies
    \begin{equation*}
        \sum_{\tau=i}^t f_\tau(\x_\tau) - \sum_{\tau = i}^t f_\tau(\u) \leq \O\left(\sqrt{\log(1+j) \sum_{\tau=i}^t f_\tau(\u)}\right)
    \end{equation*}
    for any comparator $\u \in \X$.
\end{myLemma}

The proof structure is that we will combine Lemma~\ref{lemma:adaptive-surrogate-base-regret} and Lemma~\ref{lemma:adaptive-surrogate-meta-regret} to derive Lemma~\ref{lemma:adaptive-covering-regret}, and by the property of CGC and by Cauchy-Schwarz inequality, we can extend the results to any interval, as stated in Theorem~\ref{thm:adaptive-any-interval}.

\subsection{Proof of Lemma~\ref{lemma:adaptive-surrogate-base-regret}}
\begin{proof}
    Based on Theorem~\ref{thm:sogd-T-regret}, since base algorithm (SOGD) $\Ecal_i$ starts on time $i$, notice that it can guarantee anytime regret, and we have,
    \begin{align*}
        \sum_{\tau=i}^t \inner{\gradg_t(\y_t)}{\y_{\tau, I} - \u} &{}\leq 2D\cdot \sqrt{\delta + \sum_{\tau=i}^t \norm{\nabla g_\tau(\y_\tau)}_2^2}\\
        &{} \leq  2D\cdot \sqrt{\delta + \sum_{\tau=i}^t \norm{\nabla f_\tau(\x_\tau)}_2^2}\\
        &{} \leq  2D\cdot \sqrt{\delta + 4L\sum_{\tau=i}^t f_\tau(\x_\tau)}\\
        &{} \leq  2D\cdot \sqrt{\delta} + 4D\sqrt{L\sum_{\tau=i}^t f_\tau(\x_\tau)}.
    \end{align*}
    The second inequality is because of Lemma ??. The third inequality makes use of the self-bounded property. As for the last inequality, it simply follows $\sqrt{a + b} \leq \sqrt{a} + \sqrt{b}$.
\end{proof}

\subsection{Proof of Lemma~\ref{lemma:adaptive-surrogate-meta-regret}}
\begin{proof}
    Since Ada-ML-Prod requires the regret for each expert to lie in $[-1, 1]$, we denote,
    \begin{equation*}
        \ell_t = \inner{\gradg_t(\y_t)}{\y_t} / (2GD),\  \ell_{t, i} =  \inner{\gradg_t(\y_t)}{\y_{t,i}} / (2GD),\ r_{t, i} = \ell_t - \ell_{t, i},
    \end{equation*}
    which are used in its update.

    Next we introduce some useful variables to help us prove the adaptivity of AdaMLProd to sleeping-expert setting. 
    Similar to the proof technique proposed in~\citep{ICML'15:Daniely-adaptive}, for expert $\Ecal_i$, whose active interval is defined as $[i, j]\in \mathcal{C}$, we define,
    \[ \tilde{w}_{\tau,i} = \left\{
        \begin{array}{cl}
        0 & \tau < i,\\
        1 & \tau = i,\\
        \left(\tilde{w}_{\tau-1, i}\left(1 + \eta_{\tau-1}(\hat{\ell}_{\tau-1} - \ell_{\tau-1,i})\right) \right)^{\frac{\eta_{\tau,i}}{\eta_{\tau-1, i}}} & i < \tau \leq j + 1,\\
		\tilde{w}_{j + 1, i} & \tau > j + 1.
    \end{array} \right. \]

    In addition, we use notation $\tilde{W}_t$ to denote the summation of "pseudo"-weights for all experts up to time $t$,
    \begin{equation*}
        \tilde{W}_t = \sum_{k \in [T]} \tilde{w}_{t, k}.
    \end{equation*}

    In the following part, we will try to give the lower bound and upper bound of $\tilde{W}_{t+1}$. The main techniques stem from~\citep{COLT'14:second-order-Hedge}.
    We argue that, for expert-algortim $\Ecal_i$, whose active interval is defined as $[i, j]\in \mathcal{C}$, for $t \in [i, j]$, $\ln \tilde{w}_{t+1, i}$ can be bounded as,
    \begin{equation}
        \label{eq:adamlprod-lnw-lower-bound}
        \ln \tilde{w}_{t+1, i} \geq \eta_{t + 1, i} \sum_{\tau=i}^{t} (r_{\tau, i} - \eta_{\tau,i} r_{\tau,i}^2).
    \end{equation}

    We prove the preceding inequality by induction on $t$. When $u = i$, we the above inequality holds(we assume $r_{i -1} = 0$). When $u = i + 1$, by definition, 
    \begin{equation*}
        \ln(\tilde{w}_{i+1, i}) = \frac{\eta_{i+1, i}}{\eta_{i, i}}\ln \left(1 + \eta_i r_{i, i}\right) \geq \frac{\eta_{i+1, i}}{\eta_{i, i}}\left(\eta_i r_{i, i} - \eta_i^2r_{i,i}^2\right) = \eta_{i+1, i}(r_{i, i} - \eta_{i}r_{i,i}^2),
    \end{equation*}
    where the inequality is because of $\ln(1 + x) \geq x - x^2, \forall x \geq -1/2$.

    We assume that, for $u \leq t - 1$, 
    \begin{equation*}
        \ln \tilde{w}_{u, i} \geq \eta_{u, i} \sum_{\tau=i}^{u-1} (r_{\tau, i} - \eta_{\tau,i} r_{\tau,i}^2).
    \end{equation*}

    For $u = t + 1$,
    \begin{align*}
		\ln \tilde{w}_{t+1, i} &{}=\frac{\eta_{t + 1, i}}{\eta_{t, i}} \left(\ln \tilde{w}_{t, i} + \ln \left(1 + \eta_{t, i} r_{t, i}\right) \right)\\
		&{}\geq \frac{\eta_{t + 1, i}}{\eta_{t, i}} \left(\ln \tilde{w}_{t, i} + \eta_{t, i} r_{t, i} - \eta_{t, i}^2 r_{t, i}^2 \right)\\
		&{}= \frac{\eta_{t + 1, i}}{\eta_{t, i}} \ln \tilde{w}_{t, i} + \eta_{t + 1, i}\left(r_{t,i} - \eta_{t, i} r_{t, i}^2\right)\\
		&{}\geq \frac{\eta_{t + 1, i}}{\eta_{t, i}} \left(\eta_{t, i} \sum_{\tau=i}^{t - 1} (r_{\tau, i} - \eta_{\tau,i} r_{\tau,i}^2) \right)+ \eta_{t + 1, i}\left(r_{t,i} - \eta_{t, i} r_{t, i}^2\right)\\
		&{}= \eta_{t + 1, i} \sum_{\tau=i}^{t} (r_{\tau, i} - \eta_{\tau,i} r_{\tau,i}^2).
	\end{align*}
    The first inequality again makes use of $\ln(1 + x) \geq x - x^2, \forall x \geq -1/2$. The second inequality is by induction.
    The lower bound of $\tilde{W}_{t+1}$ can be given by $\ln \tilde{w}_{t+1, i} \leq \ln \tilde{W}_{t+1}$. Then, we try to upper bound $\tilde{W}_{t+1}$ as,

    \begin{align}
        \label{eq:AdaMLProd-W-before-bound}
		\tilde{W}_{t+1} = \sum_{k \in [T]} \tilde{w}_{t+1, k} &{} = \sum_{k \in [T]:i_k = t+1} \tilde{w}_{t+1, k} + \sum_{k\in [T]: i_k \leq t} \tilde{w}_{t+1, k} \notag\\
		&{} = 1 + \sum_{k\in [T]:i_k \leq t} \tilde{w}_{t+1, k},
	\end{align}
    where we denote, for expert-algorithm $\Ecal_k$, its active interval is $[i_k, j_k]$. The second inequality is because for Compact Geometric Cover, at each round, there is only one new expert-algorithm initialized.

    For the second term in the preceding equality (for simplicity we omit the indicator that $k \in [T]$):
	\begin{align}
		\sum_{k:i_k \leq t} \tilde{w}_{t+1, k} &= \sum_{k: t \in [i_k, j_k]} \tilde{w}_{t+1, k} +  \sum_{k:t > j_k} \tilde{w}_{t+1, k}\notag \\
		&{}\leq \sum_{k: t \in [i_k, j_k]} \left( (\tilde{w}_{t+1, k})^{\frac{\eta_{t,k}}{\eta_{t+1, k}}} + \frac{1}{e} \left(\frac{\eta_{t,k}}{\eta_{t+1, k}} - 1 \right) \right)+  \sum_{k:t > j_k} \tilde{w}_{t+1, k}\notag \\
		&{}= \sum_{k: t \in [i_k, j_k]} \tilde{w}_{t,k}(1 +\eta_{t,k} r_{t,k}) + \frac{1}{e} \left(\frac{\eta_{t,k}}{\eta_{t+1, k}} - 1 \right) + \sum_{k:t > j_k} \tilde{w}_{t, k}\notag\\
		&{}= \tilde{W}_t + \underbrace{\sum_{k: t \in [i_k, j_k]} \eta_{t, k} \tilde{w}_{t,k}r_{t,k}}_{= 0} + \sum_{k: t \in [i_k, j_k]} \frac{1}{e} \left(\frac{\eta_{t,k}}{\eta_{t+1, k}} - 1 \right). \label{eq:AdaMLProd-W-w-bound}
	\end{align}
    The first ienquality is by the update rule and Lemma~\ref{lemma:second-order-hedge-weight-relation}. The second equality holds by the definition of $\tilde{w}_{t+1, k}$, where we do not update the weight because $t + 1 > j_k + 1$ and thus $\tilde{w}_{t+1, k} = \tilde{w}_{t, k}$. It is worth noticing that, the second term in the third equality equals to $0$ because of the forecasting rule and $\tilde{w}_{t, k} = w_{t, k}, \forall k: t \in[i_k, j_k]$,
    \begin{equation*}
        \sum_{k: t \in [i_k, j_k]} \eta_{t, k} \tilde{w}_{t,k}r_{t,k} = \left( \sum_{k: t \in [i_k, j_k]}\eta_{t, k} w_{t,k}\right) \sum_{k: t \in [i_k, j_k]} p_{t, k}(\ell_t - \ell_{t, k}) = 0.
    \end{equation*}
    Combining~\eqref{eq:AdaMLProd-W-before-bound} and~\eqref{eq:AdaMLProd-W-w-bound} gives,
    \begin{equation*}
        \tilde{W}_{t+1} \leq 1 + \tilde{W}_t + \frac{1}{e} \sum_{k: t \in [i_k, j_k]} \left(\frac{\eta_{t,k}}{\eta_{t+1, k}} - 1 \right).
    \end{equation*}
    Further by induction and notice that $\tilde{W}_1 = 1$, $\tilde{W}_{t+1}$ can be bounded as,
    \begin{equation}
        \label{eq:AdaMLProd-W-before-tune-ratio}
        \tilde{W}_{t+1} \leq 1 +  t + \frac{1}{e} \sum_{k \in [t]} \underbrace{\sum_{\tau = i_k}^{t \wedge j_k} \left(\frac{\eta_{\tau, k}}{\eta_{\tau + 1, k}} - 1\right)}_{\text{Term A}},
    \end{equation}
    where we denote $\alpha \wedge \beta = \min \{\alpha, \beta\}$.

    We now turn to analyze Term A.~\citet{COLT'14:second-order-Hedge} has analyzed it under static regret setting. For the sake of completeness, we here present the proof for it.
    For any $k \in [t]$, for any $\tau \in [i_k, t \wedge j_k]$, the relationship between $\eta_{\tau, k}$ and $\eta_{\tau + 1, k}$ can be considered as three cases, 
    \begin{itemize}
        \item $\eta_{\tau, k} = \eta_{\tau + 1, k} = 1/2,$
        \item 
        $
            \eta_{\tau + 1, k} =  \sqrt{\gamma_k/(1 + \sum_{u=i_k}^{\tau} r_{u, k}^2)} < \eta_{\tau, k} = \frac{1}{2},
        $
        \item $\eta_{\tau + 1, k} \leq \eta_{\tau, k} < 1/2.$
    \end{itemize}

    In all cases, the ratio $\eta_{\tau, k} / \eta_{\tau + 1, k} - 1$ can be bounded as,
    \begin{align}
        \sum_{\tau = i_k}^{t \wedge j_k} \left( \frac{\eta_{\tau, k}}{\eta_{\tau + 1, k}} - 1\right) &{}\leq  \sum_{\tau = i_k}^{t \wedge j_k} \left(\sqrt{\frac{1 + \sum_{u=i_k}^{\tau} r_{u, k}^2}{1 + \sum_{u=i_k}^{\tau - 1} r_{u, k}^2}} - 1\right) \notag\\
        &{}=\sum_{\tau = i_k}^{t \wedge j_k} \left( \sqrt{\frac{r_{\tau, k}^2}{1 + \sum_{u=i_k}^{\tau - 1} r_{u, k}^2} + 1} - 1 \right)\notag\\
        &{}\leq \frac{1}{2} \sum_{\tau = i_k}^{t \wedge j_k} \frac{r_{\tau, k}^2}{1 + \sum_{u=i_k}^{\tau - 1} r_{u, k}^2}\notag\\
        &{}\leq \frac{1}{2} \left( 1 + \ln\left(1 + \sum_{u=i_k}^{t \wedge j_k} r_{u, k}^2\right)\right) - \ln(1)\notag\\
        &{}\leq \frac{1}{2} \left( 1 + \ln(1 + t)\right). \label{eq:AdaMLProd-tune-ratio}
    \end{align}
    The second inequality makes use of $\sqrt{1 + x} \leq 1 + x/2$. The third inequality follows Lemma~\ref{lemma:adamlprod-self-confident} with the choice of $f(x) = 1/x$.

    Substituting~\eqref{eq:AdaMLProd-tune-ratio} into~\eqref{eq:AdaMLProd-W-before-tune-ratio}, we can upper bound $\tilde{W}_{t+1}$ as,
    \begin{align*}
        \tilde{W}_{t+1} \leq  1 + t +\frac{1}{2e}t\left(1 + \ln(1+t)\right) \leq (1+t)(1 + \ln (1 +t )) \leq (1+t)^2.
    \end{align*}
    The second ienquality is because of $t(1 + \ln(1+t))/(2e) \leq (1+t)(1 + \ln(1+t)), \forall  t \geq 1$.

    Combining the upper bound and lower bound of $\ln \tilde{W}_{t+1}$, we can have
    \begin{equation*}
        \eta_{t + 1, i} \sum_{\tau=i}^{t} (r_{\tau, i} - \eta_{\tau,i} r_{\tau,i}^2) \leq  \ln \tilde{w}_{t+1, i} \leq \ln \tilde{W}_{t+1} \leq 2\ln(1+t).
    \end{equation*}

    Rearranging the preceding inequality gives
    \begin{align}
        \sum_{\tau=i}^{t}r_{\tau, i} &{}\leq \sum_{\tau=i}^t \eta_{\tau,i}r_{\tau,i}^2 + \frac{2\ln(1+t)}{\eta_{t+1, i}} \notag\\
        &{} \leq 2\sqrt{\gamma_i} \sqrt{1 + \sum_{\tau = i}^t  r_{\tau, i}^2}   + \frac{2\ln(1+t)}{\eta_{t+1, i}} \label{eq:adamlprod-gamma-tuning}\\
        &{} \leq  \frac{2\ln(1+t) + 2\gamma_i}{\sqrt{\gamma_i}} \sqrt{1 + \sum_{\tau = i}^t  r_{\tau, i}^2}  + 4\ln(1+t) + 4\gamma_i\label{eq:pd-adamlprod-refer}\\
        &{} \leq 4\sqrt{\ln(1 + j)}\sqrt{1 + \sum_{\tau = i}^t  r_{\tau, i}^2} + 8\ln(1 + j).\label{eq:adamlprod-interval-meta-regret}
    \end{align}
    The second inequality is by Lemma~\ref{lemma:adamlprod-self-confident} and choose $f(x) = 1/\sqrt{x}$. As for the third inequality, there are two cases to be considered:
    \begin{itemize}
        \item If $\sqrt{1 + \sum_{\tau = i}^t  r_{\tau, i}^2 } > 2\sqrt{\gamma_i}$, then~\eqref{eq:adamlprod-gamma-tuning} is no greater than
        \begin{equation*}
            2\sqrt{\gamma_i} \sqrt{1 + \sum_{\tau = i}^t  r_{\tau, i}^2} + \frac{2\ln(1+t)}{\sqrt{\gamma_i}} \sqrt{1 + \sum_{\tau = i}^t  r_{\tau, i}^2}.
        \end{equation*}
        \item If $\sqrt{1 + \sum_{\tau = i}^t  r_{\tau, i}^2 } \leq 2\sqrt{\gamma_i}$, then $\eta_{t+1, i} = 1/2$, and~\eqref{eq:adamlprod-gamma-tuning} is bounded by,
        \begin{equation*}
            4\gamma_i + 4\ln(1+t)
        \end{equation*}
    \end{itemize}
    Therefore,~\eqref{eq:adamlprod-gamma-tuning} is no greater than the sum of the preceding two terms, which leads to the third inequality. The forth inequality is by the setting of $\gamma_i = \ln(1+j)$ and $\ln(1+t) \leq \ln(1+j)$.

    Finally, following~\eqref{eq:adamlprod-interval-meta-regret},
    \begin{align}
        & \sum_{\tau = i}^t \inner{\gradg_t(\y_t)}{\y_t - \y_{t, i}} \\
        &{}= 2GD\cdot\sum_{\tau=i}^{t}r_{\tau, i}\notag \\
        &{}\leq 8GD\sqrt{\ln(1 + j)}\sqrt{1 + \sum_{\tau = i}^t  r_{\tau, i}^2} + 16GD\ln(1+j)\notag\\
        &{} \leq 8GD\sqrt{\ln(1+j)\sum_{\tau = i}^t  r_{\tau, i}^2} + 16GD\ln(1+j) + 8GD\sqrt{\ln(1+j)}\notag\\
        &{} =4\sqrt{\ln(1+j)\sum_{\tau = i}^t  \left(\inner{\gradg_t(\y_t)}{\y_t - \y_{t, i}}\right)^2}+ 16GD\ln(1+j) + 8GD\sqrt{\ln(1+j)}\notag\\
        &{}\leq 8D\sqrt{L\ln(1+j)\sum_{\tau = i}^t f_t(\x_t)}+ 16GD\ln(1+j) + 8GD\sqrt{\ln(1+j)}\label{eq:pd-adamlprod-meta-refer}
    \end{align}
    The second inequality makes use of $\sqrt{a + b} \leq \sqrt{a} + \sqrt{b}$. The last inequality utilizes Lemma ?? and the self-bounded property of smooth function, similar to the proof of Theorem~\ref{thm:Adaptive-surrogate-base-regret}.
\end{proof}

\subsection{Proof of Lemma~\ref{lemma:adaptive-covering-regret}}
\begin{proof}
    Similar to the proof of Theorem~\ref{thm:small-loss-dynamic-regret}, we begin the proof with
    \begin{align}
        &{}\sum_{\tau=i}^t f_\tau(\x_\tau) - \sum_{t=i}^t f_\tau(\u) \notag \\
        &{}\leq \sum_{\tau=i}^t g_\tau(\y_\tau) - \sum_{t=i}^t g_\tau(\u) \notag \\
        &{}\leq  \sum_{\tau=i}^t \inner{\nabla g_\tau(\y_\tau)}{\y_\tau - \u} \notag \\
        &{}=\underbrace{ \sum_{\tau=i}^t \inner{\nabla g_\tau(\y_\tau)}{\y_\tau - \y_{\tau, i}}}_{\meta} + \underbrace{ \sum_{\tau=i}^t \inner{\nabla g_\tau(\y_{\tau})}{\y_{\tau, i} - \u}}_{\base}. \label{eq:adaptive-before-plug}
    \end{align}
    \paragraph{Upper bound of base-regret.}
    By Lemma~\ref{lemma:adaptive-surrogate-base-regret}, we can directly bound base-regret as,
    \begin{equation}
        \label{eq:adaptive-base-regret}
        \sum_{\tau=i}^t \inner{\nabla g_\tau(\y_\tau)}{\y_{\tau, i} - \u} \leq 2D\sqrt{\delta} + 4D\sqrt{L\sum_{\tau=i}^t f_\tau(\x_\tau)} 
    \end{equation}
    \paragraph{Upper bound of meta-regret.}
    By Lemma~\ref{lemma:adaptive-surrogate-meta-regret}, the direct application will lead to
    \begin{equation}
        \label{eq:adaptive-meta-regret}
        \sum_{\tau = i}^t \inner{\gradg_\tau(\y_\tau)}{\y_\tau - \y_{\tau, i}} \leq 8D\sqrt{L\ln(1+j)\sum_{\tau = i}^t f_\tau(\x_\tau)}+ 16GD\ln(1+j) + 8GD\sqrt{\ln(1+j)}.
    \end{equation}
    \paragraph{Upper bound of adaptive regret.}
    Replacing the base-regret and meta-regret in~\eqref{eq:adaptive-before-plug} with~\eqref{eq:adaptive-base-regret} and~\eqref{eq:adaptive-meta-regret}, further we can have,
    \begin{align*}
        &{}\sum_{\tau=i}^t f_\tau(\x_\tau) - \sum_{t=i}^t f_\tau(\u) \\
        &{} \leq \left(8D\sqrt{L\ln(1+j)} + 4D\sqrt{L}\right)\sqrt{\sum_{\tau = i}^t f_t(\x_t)}+ 16GD\ln(1+j) + 8GD\sqrt{\ln(1+j)} + 2D\sqrt{\delta}.
    \end{align*}

    By Lemma~\ref{lemma:substitute-F_T}, we can rewrite the adaptive regret into
    \begin{align*}
        &{}\sum_{\tau=i}^t f_\tau(\x_\tau) - \sum_{t=i}^t f_\tau(\u) \\
        &{} \leq \left(8D\sqrt{L\ln(1+j)} + 4D\sqrt{L}\right)\sqrt{\sum_{\tau = i}^t f_\tau(\u) + 16GD\ln(1+j) + 8GD\sqrt{\ln(1+j)} + 2D\sqrt{\delta}}\\
        &{}+ 16GD\ln(1+j) + 8GD\sqrt{\ln(1+j)} + 2D\sqrt{\delta} + (8D\sqrt{L\ln(1+j)} + 4D\sqrt{L})^2\\
        &{} \leq  \left(8D\sqrt{L\ln(1+j)} + 4D\sqrt{L}\right)\sqrt{\sum_{\tau = i}^t f_\tau(\u)} \\
        &{} + 24GD\ln(1+j) + 12GD\sqrt{\ln(1+j)} + 4D\sqrt{\delta} + \frac{3}{2}(8D\sqrt{L\ln(1+j)} + 4D\sqrt{L})^2,
    \end{align*}
    where the last ienquality makes use of $\sqrt{a + b} \leq \sqrt{a} + \sqrt{b}$ and $\sqrt{ab} \leq \frac{a^2 + b^2}{2}$. The preceding arguments finish the proof.
\end{proof}

\subsection{Proof of Theorem~\ref{thm:adaptive-any-interval}}
\begin{proof}
    First, we define the following notations,
    \begin{align*}
        \alpha(t)&{} = 24GD\ln(1+t) + 12GD\sqrt{\ln(1+t)} + 4D\sqrt{\delta} + \frac{3}{2}(8D\sqrt{L\ln(1+t)} + 4D\sqrt{L})^2,\\
        \beta(t) &{} = 8D\sqrt{L\ln(1+t)} + 4D\sqrt{L}.
    \end{align*}
    Then, for any covering interval $[i, j] \in \mathcal{C}$, Lemma~\ref{lemma:adaptive-covering-regret} can be presented as,
    \begin{equation*}
        \sum_{\tau=i}^j f_\tau(\x_\tau) - \sum_{\tau = i}^j f_\tau(u) \leq \alpha(j) + \beta(j)\sqrt{F_{[i, j]}}.
    \end{equation*}

    By Lemma~\ref{lemma:CGC number}, we know that, any interval $I=[q,s]\subseteq[T]$ can be decomposed into several consecutive covering intervals. We continue the notations used in Lemma~\ref{lemma:CGC number}. Assume $I$ can be decomposed into $v$ covering intervals, such that,
    \begin{equation*}
        I_1=[i_1, i_2 - 1],\  I_2 = [i_2, i_3 - 1],\  \dots , I_v = [i_v, i_{v+1} - 1] \in \mathcal{C}
    \end{equation*}
    and, 
    \begin{equation*}
        i_1 = q,\  i_v\leq s \leq i_{v+1} - 1, \text{and } v \leq \lceil \log_2(s-q+2) \rceil
    \end{equation*}
    For the first $v-1$ intervals, according to Lemma~\ref{lemma:adaptive-covering-regret}, the regret can be bounded as,
    \begin{align}
        \sum_{\tau=i_k}^{i_{k+1} -1} f_\tau(\x_\tau) - \sum_{\tau=i_k}^{i_{k+1} -1} f_\tau(u) &{}\leq \alpha(i_{k+1} - 1) + \beta(i_{k+1} - 1)\sqrt{F_{I_k}} \notag \\
        &{} \leq\alpha(s) + \beta(s)\sqrt{F_{I_k}} \ , \forall k \in [v-1].\label{eq:adaptive-before-cauchy}
    \end{align}

    For the last interval, we can bound it as,
    \begin{equation*}
        \sum_{\tau=i_v}^{s} f_\tau(\x_\tau) - \sum_{\tau=i_k}^{s} f_\tau(u) \leq \alpha(2s) + \beta(2s)\sqrt{F_{[i_{v}, t]}}.
    \end{equation*}
    The inequality is because, by the construction of Compact Geometric Cover, we know that $i_{v+1} \leq 2i_{v}$, thus, for any $t \in [i_v, i_{v+1} - 1]$, we have $i_{v+1} - 1 \leq 2t$. Also, notice that $\alpha(\cdot), \beta(\cdot)$ is monotonically increasing function.

    Combining $v$ intervals together, we have
    \begin{align*}
        \sum_{\tau=q}^s f_\tau(\x_\tau) - \sum_{\tau = q}^s f_\tau(\u) &{}\leq v\alpha(2s) + \beta(2s)\left(\sum_{k=1}^{v-1}\sqrt{F_{I_k}} + \sqrt{F_{[i_v, t]}}\right)\\
        &{} \leq v\alpha(2s) + \beta(2s)\sqrt{vF_I},
    \end{align*}
    where the last inequality makes use of Cauchy-Schwarz inequality.

    The preceding arguments result in small-loss adaptive regret, but suffer an additional $\O(\sqrt{\log(s-q)})$ term. However, if we consider minimax adaptive regret, then we can avoid using Cauchy-Schwarz inequality to derive the desired bound, and hence save the additional term.

    Reconsidering~\eqref{eq:adaptive-before-cauchy}, by Assumptions~\ref{assumption:bounded-gradient},~\ref{assumption:bounded-domain} and~\ref{assumption:non-negative}, $f_t(\u) \in [0, GD], \forall t \in [T], \forall \u \in \X$, its minimax form will be,
    \begin{equation*}
        \sum_{\tau=i_k}^{i_{k+1} -1} f_\tau(\x_\tau) - \sum_{\tau=i_k}^{i_{k+1} -1} f_\tau(u) \leq \alpha(s) + \beta(s)\sqrt{GD|I_k|},\ \forall k \in [v-1]
    \end{equation*}

    Similarly, for the $v$-th covering interval,
    \begin{equation*}
        \sum_{\tau=i_v}^{s} f_\tau(\x_\tau) - \sum_{\tau=i_k}^{s} f_\tau(u) \leq \alpha(2s) + \beta(2s)\sqrt{GD|I|}.
    \end{equation*}
    The inequality is because we do not know the true overlap length for $I$ and $I_k$ and just can overestimate it as $|I|$.

    It is easy to verify that, the length of consecutive intervals in Compact Geometric Cover(also known as Data Streaming Cover proposed by~\citet{journal'07:Hazan-adaptive}) will be exponentially increasing. \yfnote{Do we need this lemma?}. Therefore,
    \begin{align*}
        \sum_{\tau=q}^s f_\tau(\x_\tau) - \sum_{\tau = q}^s f_\tau(\u) &{}\leq v\alpha(2s) + \beta(2s)\sqrt{GD}\left(\sum_{k=1}^{v-1}\sqrt{|I_k|} + \sqrt{|I|}\right)\\
        &{} \leq v\alpha(2s) + \beta(2s)\sqrt{GD}(\sqrt{|I|}+\sum_{i=0}^{+\infty}\sqrt{\frac{|I|}{2^i}})\\
        &{} \leq v\alpha(2s) + \frac{2\sqrt{2}-1}{\sqrt{2} - 1}\beta(2s)\sqrt{GD|I|}
    \end{align*}
    Thus, in asymptotic view, the adaptive regret for any interval $I$ with be the order of
    \begin{equation*}
        \O\left(\log|I|\log T + \sqrt{|I|\log T}\right) \leq \O\left(\sqrt{\log T (|I| + \log^2|I| \cdot \log T)}\right).
    \end{equation*}
   
    Under the minimax adaptive regret view, currently, the "optimal" order will be $\O(\sqrt{|I| \log T})$, which means the only when $|I| = \Omega(\log T)$, the guarantee will be meaningful. Therefore, $|I|$ and $\log^2|I| \cdot \log T$ will be the same order, if we treat $\O(\log\log T)$ term as constant, and the minimax adaptive regret will be of order $\O(\sqrt{|I| \log T})$.
\end{proof}
