# Supplementary material for: Efficient Methods for Non-stationary Online Learning
Source: arXiv:2309.08911 source file (2025-09-09)
Supplement: Supplementary file 2 [file appendix_preliminary.tex]

%!TEX root = ../jmlr23_projection.tex
\section{Preliminaries}
\label{sec:appendix-preliminary}
This section present preliminaries for analyzing the main theorems, including the dynamic regret of OGD and SOGD, second-order regret of Adapt-ML-Prod, self-confident tuning, and several facts of geometric covers.

\subsection{OGD and Dynamic Regret}

This part provides the dynamic regret of online gradient descent (OGD)~\citep{ICML'03:zinkvich} and scale-free online gradient descent (SOGD)~\citep{TCS'18:SOGD} from the view of online mirror descent (OMD), which is a common and powerful online learning framework. Following the analysis in~\citep{JMLR:sword++}, we can directly obtain dynamic regret of OGD and SOGD~\citep{TCS'18:SOGD} in a unified view owing to the versatility of OMD. 

Online mirror descent algorithm updates according to the following rule:
\begin{equation}
    \label{eq:OMD-update-rule}
    \x_{t+1} = {}  \argmin_{\x \in \X}~\eta_t \inner{\nabla f_{t}(\x_{t})}{\x} + \D_{\Rcal}(\x,\x_{t}),
\end{equation}
where $\eta_t > 0$ is the time-varying step size, and $\D_{\Rcal}(\cdot, \cdot)$ is the Bregman divergence induced by the regularizer function $\Rcal(\cdot)$ defined as $\D_{\Rcal}(\x, \y) = \Rcal(\x) - \Rcal(\y) - \inner{\nabla \Rcal(\y)}{\x - \y}$. OMD following dynamic regret guarantee~\citep{JMLR:sword++}.

\begin{myThm}[Theorem 1 of~\citet{JMLR:sword++}]
    \label{thm:omd-dynamic-regret}
    Suppose that the regularizer $\Rcal: \X \mapsto \R$ is  1-strongly convex with respect to the norm $\|\cdot\|$. The dynamic regret of Optimistic Mirror Descent (OMD) whose update rule specified in~\eqref{eq:OMD-update-rule} is bounded as follows: 
\begin{align*}
\sum_{t=1}^{T} f_t(\x_t) - \sum_{t=1}^{T} f_t(\u_t) \leq \sum_{t=1}^{T}\eta_t \norm{\nabla f_t(\x_t)}_*^2 {} &{}+  \sum_{t=1}^{T} \frac{1}{\eta_t} \Big( \Div{\u_t}{\x_t} - \Div{\u_t}{\x_{t+1}}\Big) \\
&{} -  \sum_{t=1}^{T} \frac{1}{\eta_t}\Div{\x_{t+1}}{\x_t},
\end{align*}
which holds for any comparator sequence $\u_1,\ldots,\u_T \in \X$.
\end{myThm}

Choosing $\Rcal(\x) = \frac{1}{2}\norm{\x}_2^2$ will lead to the update form of online gradient descent used as base learners in our algorithm:
\begin{equation}
    \label{eq:OGD-update-rule}
    \x_{t+1} = {}  \argmin_{\x \in \X}~\eta_t \inner{\nabla f_{t}(\x_{t})}{\x} + \frac{1}{2} \norm{\x - \x_t}^2_2,
\end{equation}
where the Bregman divergence becomes $ \D_{\Rcal}(\x,\x_{t}) = \frac{1}{2}\norm{\x-\x_t}_2^2$ w.r.t. the choice of regularizer. 

We proceed to show the dynamic regret of online gradient descent (OGD),

\begin{myThm}
    \label{thm:ogd-dynamic-regret}
    Under Assumption~\ref{assumption:bounded-domain}, by choosing static step size $\eta_t = \eta > 0$, Online Gradient Descent defined in equation~\eqref{eq:OGD-update-rule} satisfies:
    \begin{equation*}
        \sum_{t=1}^{T} f_t(\x_t) - \sum_{t=1}^{T} f_t(\u_t) \leq \frac{7D^2}{4\eta} + \frac{D}{\eta}\sum_{t=2}^T \norm{\u_{t-1} - \u_2}_2 + \eta \sum_{t=1}^T \norm{\nabla f_t(\x_t)}_2^2
    \end{equation*}
    for any comparator sequence $\u_1,\ldots,\u_T \in \X$. 
\end{myThm}
\begin{proof}
    Applying Theorem~\ref{thm:omd-dynamic-regret} with the choices of $\Rcal(\x) = \frac{1}{2} \norm{\x}_2^2$ and fixed step size $\eta_t = \eta > 0$ gives:
    \begin{align*}
        {} & \sum_{t=1}^{T} f_t(\x_t) - \sum_{t=1}^{T} f_t(\u_t)\\
   \leq {} &  \frac{1}{2\eta} \sum_{t=1}^{T} \Big( \norm{\u_t - \x_t}_2^2 - \norm{\u_t - \x_{t+1}}_2^2\Big) + \eta \sum_{t=1}^{T} \norm{\nabla f_t(\x_t)}_2^2 - \frac{1}{2\eta} \sum_{t=1}^T \norm{\x_t - \x_{t+1}}_2^2\\
   \leq {} &  \frac{1}{2\eta} \sum_{t=1}^{T} \left(\norm{\x_t}_2^2 - \norm{\x_{t+1}}_2^2\right) + \frac{1}{\eta} \sum_{t=1}^T \left(\x_{t+1} - \x_{t}\right)^\top \u_t + \eta \sum_{t=1}^{T} \norm{\nabla f_t(\x_t)}_2^2 \\
   \leq {} &  \frac{1}{2\eta}\norm{\x_1}_2^2 + \frac{1}{\eta}\left(\x_{T+1}^\top \u_T - \x_1^\top \u_1 \right) + \frac{1}{\eta}\sum_{t=2}^T(\u_{t-1} - \u_t)^\top \x_t + \eta \sum_{t=1}^{T} \norm{\nabla f_t(\x_t)}_2^2\\
   \leq {} &  \frac{7D^2}{4\eta} + \frac{D}{\eta}\sum_{t=2}^T \norm{\u_{t-1} - \u_2}_2 + \eta \sum_{t=1}^{T} \norm{\nabla f_t(\x_t)}_2^2\\
    \end{align*}
    where the last inequality is due to:
    \begin{align*}
        \norm{\x_1}_2^2 &{}= \norm{\x_1 - \boldsymbol{0}}_2^2 \leq D^2,\\
        \x_{T+1}^\top \u_T &{}\leq \norm{\x_{T+1}}_2 \cdot \norm{\u_T}_2 = D^2,\\
        -\x_1^\top\u_1&{}\leq \frac{1}{4}\norm{\x_1 - \u_1}_2^2 \leq \frac{1}{4}D^2\\
        (\u_{t-1} - \u_t)^\top \x_t &{} \leq \norm{\u_{t-1} - \u_t}_2 \cdot \norm{\x_t}_2 \leq D\norm{\u_{t-1} - \u_t}_2
    \end{align*}
\end{proof}

\subsection{Adapt-ML-Prod and Second-Order Regret}
In this part, we will introduce an algorithm named Adapt-ML-Prod~\citep{COLT'14:second-order-Hedge}, which equips with a second-order regret bound for any expert and is one of the key ingredients for designing our adaptive algorithms. Consider the standard PEA setting. There are $K$ experts, and at each round, the learner is required to provide a probability distribution $\p_t \in \Delta(K)$ over the $K$ experts and then receives a loss vector $\ellb_t \in [0,1]^K$ revealed from the environments and suffers $\p_t^\top \ellb_t$. 

Adapt-ML-Prod will maintain and update the weight and learning rate for every tracked expert (say the $i$-th expert) as:
\begin{align}
    \eta_{t, i}&{} = \min \left\{\frac{1}{2}, \sqrt{\frac{\gamma_i}{1 + \sum_{\tau=1}^{t-1} (\p_\tau^\top \ellb_\tau - \ell_{\tau, i} )^2}} \right\}, \label{eq:ada-ml-prod learning rate}\\
    w_{t, i} &{} =  \left(w_{t-1,i} \left(1 + \eta_{t-1,i} (\p_t^\top \ellb_{t-1} - \ell_{t-1, i})\right) \right)^{\frac{\eta_{t, i}}{\eta_{t-1, i}}}. \label{eq:ada-ml-prod weight}
\end{align}

When it is time to predict, Adapt-ML-Prod will generate its decision based on the aforementioned weight and learning rate in the following style:
\begin{equation*}
    p_{t, i} = \frac{\eta_{t, i} \cdot w_{t, i}}{ \sum_{j=1}^K \eta_{t, j} \cdot w_{t, j}}
\end{equation*}

The advantage of using Adapt-ML-Prod is that it has second-order excess risk regret bound guarantee, which can further relate the gradient and the function value for smooth function. For static regret, the property of Adapt-ML-Prod can be summarized into the below theorem:
\begin{myThm}[Corollary 4 of~\citet{COLT'14:second-order-Hedge}]
    With uniform initialization of weight $w_{1,i} = 1/K, \forall i \in [K]$ in equation~\eqref{eq:ada-ml-prod weight} and $\gamma_i = \ln K, \forall i \in [K]$ in equation~\eqref{eq:ada-ml-prod learning rate}, Adapt-ML-Prod satisfies:
    \begin{align*}
        \sum_{t=1}^T \p_t^\top\ellb_t - \sum_{t=1}^T \ell_{t, i} \leq \frac{C_{K, T}}{\sqrt{\ln K}}\sqrt{1 + \sum_{t=1}^T (\p_t^\top \ellb_t - \ell_{t, i})^2} + C_{K, T}
    \end{align*}
    for any expert $i$, where $C_{K, T} = 3\ln K + \ln \left(1 + \frac{K}{2e}(1 + \ln (1+T))\right)$.%\yfnote{Maybe here just use O-notation to avoid new definition}
\end{myThm}

It is worthy pointing out that~\citet{ICML19:Zhang-Adaptive-Smooth} use the  AdaNormalHedge algorithm~\citep{COLT'15:Luo-AdaNormalHedge} in the design of adaptive algorithm and can also achieve problem-dependent adaptive regret bound. However, AdaNormalHedge can only enjoy the \emph{first-order} regret bound, which is not thus more difficult to establish small-loss type bound when the meta-algorithm is restricted to use the surrogate loss.

\subsection{Self-Confident Tuning}
\label{sec:appendix-self-condident-tuning}
\citet{tcs'18:orabona-scale-free} have analyzed the regret bound of SOGD, for the sake of completeness, we provide the analysis of it under the framework of OMD. The derivation of regret bound for SOGD can be seen as the process of self-confident learning rate tuning under OMD framework.
\begin{myThm}
    \label{thm:sogd-T-regret}
    Under assumption~\ref{assumption:bounded-gradient} and~\ref{assumption:bounded-domain}, the OMD algorithm defined in equation~\eqref{eq:OMD-update-rule} with the choices of regularizer $\Rcal(\x) = \frac{1}{2}\norm{\x}_2^2$ and the time-varying learning rate defined as:
    \begin{equation*}
        \eta_{t} = \frac{D/2}{\sqrt{\delta + \sum_{\tau=1}^{t-1} \|\nabla f_t(\x_t)\|_2^2}}
    \end{equation*}
    for some $\delta > 0 $, has the following guarantee:
    \begin{equation*}
        \sum_{t=1}^T f_t(\x_t) - \sum_{t=1}^T f_t(\u) \leq 2D\cdot \sqrt{\delta + \sum_{t=1}^T \norm{\nabla f_t(\x_t)}_2^2},
    \end{equation*}
    where $\u \in \X$ can be any comparator.
\end{myThm}
\begin{proof}
    We start the proof with the application of Theorem~\ref{thm:omd-dynamic-regret}, for any fixed comparator $\u \in \X$:
    \begin{align}
        {} & \sum_{t=1}^{T} f_t(\x_t) - \sum_{t=1}^{T} f_t(\u_t) \notag \\
        \leq {} & \sum_{t=1}^{T} \frac{1}{2\eta_t} \Big( \norm{\u - \x_t}_2^2 - \norm{\u - \x_{t+1}}_2^2\Big) +  \sum_{t=1}^{T} \eta_t \norm{\nabla f_t(\x_t)}_2^2 -  \sum_{t=1}^T\frac{1}{2\eta_t} \norm{\x_t - \x_{t+1}}_2^2\notag\\
        \leq {} & \frac{1}{2\eta_1}\norm{\u - \x_1}_2^2 + \sum_{t=2}^T \left(\frac{1}{\eta_t} - \frac{1}{\eta_{t-1}}\right) \frac{\norm{\u - \x_t}_2^2}{2} +  \sum_{t=1}^{T} \eta_t \norm{\nabla f_t(\x_t)}_2^2 \notag \\
        \leq {} & \frac{D^2}{2\eta_1} + \frac{D^2}{2} \sum_{t=2}^T \left(\frac{1}{\eta_t} - \frac{1}{\eta_{t-1}}\right) +  \sum_{t=1}^{T} \eta_t \norm{\nabla f_t(\x_t)}_2^2  \notag\\
        =    {} & \frac{D^2}{2\eta_T} +  \sum_{t=1}^{T} \eta_t \norm{\nabla f_t(\x_t)}_2^2 \label{eq:sogd-regret-before tuning}
    \end{align}

    Applying Lemma~\ref{lemma:self-confident} to the second term in equation~\eqref{eq:sogd-regret-before tuning} and by the definition of $\eta_T$, the regret bound becomes:
    \begin{align*}
        \sum_{t=1}^{T} f_t(\x_t) - \sum_{t=1}^{T} f_t(\u_t) &{} \leq D\cdot\sqrt{\delta + \sum_{t=1}^T \norm{\nabla f_t(\x_t)}_2^2} + D\left(\sqrt{\delta + \sum_{t=1}^T \norm{\nabla f_t(\x_t)}_2^2} - \sqrt{\delta} \right)\\
    &{}\leq  2D\cdot \sqrt{\delta + \sum_{t=1}^T \norm{\nabla f_t(\x_t)}_2^2}
    \end{align*} 
    which completes the proof.
\end{proof}

We first introduce a FTRL lemma~\cite[Corollary 7.8]{book'12:FO-book}.
\begin{myLemma}[FTRL Lemma]
\label{lemma:FTRL-Lemma}
    \begin{equation*}
        \sum_{t=1}^{T} \ell\left(\boldsymbol{x}_{t}\right)-\sum_{t=1}^{T} \ell_{t}(\boldsymbol{u}) \leq \frac{\psi(\boldsymbol{u})-\min _{\boldsymbol{x} \in V} \psi(\boldsymbol{x})}{\eta_{T-1}}+\frac{1}{2 \mu} \sum_{t=1}^{T} \eta_{t-1}\left\|\boldsymbol{g}_{t}\right\|_{\star}^{2}
    \end{equation*}
\end{myLemma}

Based on the previous Lemma, we can derive self-confident tuning hedge,
\begin{myLemma}
    \label{lemma:self-tuning-hedge}
    There exists the static regret bound:
    \begin{equation*}
        \sum_{t=1}^T \inner{\p_t}{ \ellb_t} -  \sum_{t=1}^T \ell_{t, i} \leq 3\sqrt{\ln N \cdot \left(1 + \sum_{t=1}^T\norm{\ellb_t}_{\infty}^2 \right) } +\frac{G^2}{2}\sqrt{\ln N}
    \end{equation*}
    for any $i \in [N]$.
\end{myLemma}

\subsection{Facts on Geometric Covers}
\begin{myLemma}[Lemma 10 of~\citet{ICML19:Zhang-Adaptive-Smooth}]
    \label{lemma:CGC number}
    Let $[r, s] \subseteq [T]$ be an arbitrary interval. Then, we can find a sequence of consecutive intervals in Compact Geometric Cover:
    \begin{equation*}
        I_1=[i_1, i_2 - 1],\  I_2 = [i_2, i_3 - 1],\  \dots , I_v = [i_v, i_{v+1} - 1] \in \mathcal{C}
    \end{equation*}
    such that
    \begin{equation*}
        i_1 = r,\  i_v\leq s \leq i_{v+1} - 1, \text{and } v \leq \lceil \log_2(s-r+2) \rceil
    \end{equation*}
\end{myLemma}

Lemma~\ref{lemma:CGC number} can be extend to Problem-Dependent Geometric Cover:
\begin{myLemma}[Lemma 11 of~\citet{ICML19:Zhang-Adaptive-Smooth}]
    \label{lemma:pcgc-number}
    Let $[s_p, s_q] \subseteq [T]$ be an arbitrary that starts from an marker $s_p$ and ends at another marker $s_q$. Then, we can find a sequence of consecutive intervals
    \begin{equation*}
        I_1=[s_{i_1}, s_{i_2} - 1],\  I_2 = [s_{i_2}, s_{i_3} - 1],\  \dots , I_v = [s_{i_v}, s_{i_{v+1}} - 1] \in \tilde{\mathcal{C}}
    \end{equation*}
    such that
    \begin{equation*}
        i_1 = p,\  i_v\leq q < i_{v+1}, \text{and } v \leq \lceil \log_2(q-p+2) \rceil
    \end{equation*}
\end{myLemma}
